# Supplementary material for: Proposal for demonstrating the Hong-Ou-Mandel effect with matter waves
Source: arXiv:1312.3933 source file (2014-04-27)
Supplement: Supplementary file 1 [file HOM_NComms_Supplementary_resub_v3.pdf]

# Supplementary Figures

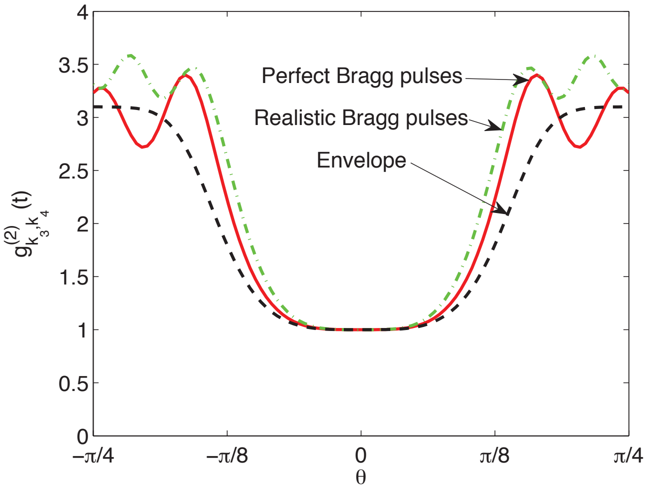


**Supplementary Figure 1: HOM dip profile from analytic treatments.** Normalised correlation function $g^{(2)}_{\mathrm{RL}}(t_4)$ between atomic populations after the $\pi$/2-pulse. The HOM dip is realised in the simplest model [equation (9)], corresponding to a uniform BEC in the undepleted pump approximation and perfect mirrors and a symmetric beam-splitter (full red line). We also consider the case of off-resonant Bragg pulses (green dot-dashed line), corresponding to the case of an asymmetric beam-splitter (see Supplementary Note 4). For comparison we plot the envelope fit of equation (14) (dashed black curve), which shows reasonable agreement with the overall shape of the dip of equation (9). For all analytic calculations, the uniform density $\rho_0$ is chosen to match the peak density of the source BEC used the numerical results of the main text. The collision duration (and a matching free-propagation time), on the other hand, is chosen to be somewhat shorter ($t_1 = 30\mu$s) in order to result in a radial rms width of the scattering halo ($\delta k_r \simeq 0.1|\mathbf{k}_0|$) that agrees with the one obtained in pure numerical simulations. While overestimating the peak mode occupancy in the scattering halo ($n_{\mathbf{k}_3}(t_1) = 0.45$), this choice of parameters optimises the overall shape of the HOM dip as a function of the widths of the normal and anomalous densities, $n_{\mathbf{k}_6}(t_1)$ and $|m_{\mathbf{k}_5,\mathbf{k}_6}(t_1)|$.

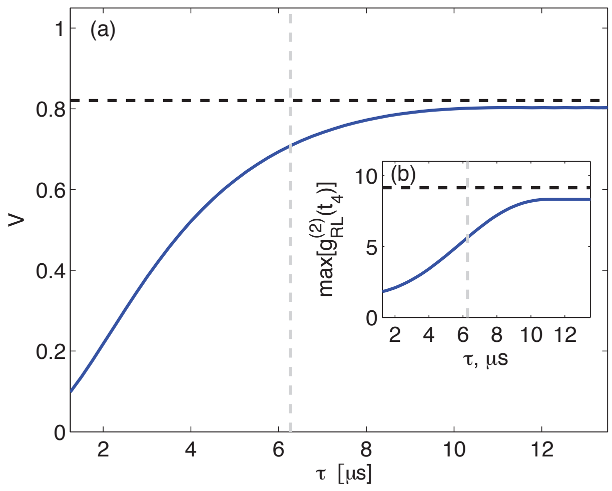


**Supplementary Figure 2: HOM dip visibility from analytic treatments.** (a) Visibility of the HOM dip as a function of pulse duration $\tau_\pi = \tau_{\pi/2} = \tau$. We compare the case of a uniform scattering halo taking into account off-resonant coupling (solid blue line) with that calculated from the full undepleted pump model (inhomogeneous scattering halo) and perfect Bragg pulses

(dashed black line). We indicate on the figure (vertical dashed line) the equivalent pulse duration for the Gaussian pulses used in the main numerical results ($\tau' = 2.5\ \mu$s), which leads to a maximum visibility of 70% ($V = 0.70$) for the case of realistic Bragg pulses, compared to 82% for the perfect case. (b) The maximum obtained $g^{(2)}_{\mathrm{RL}}(t_4)$, corresponding to $|\theta| = \pi/4$, for the case of realistic (solid blue line) and perfect (dashed black line) Bragg pulses. The perfect case corresponds to the average value $\overline{g^{(2)}_{\mathrm{RL}}(t_4)} = 2 + 1/2n_0$. Equivalent Gaussian pulse duration is again indicated (vertical dashed line) for reference.

## Supplementary Notes

**Supplementary Note 1: Model Hamiltonian in undepleted pump approximation.** We begin by considering the collision process in the Bogoliubov approximation, in which the atomic field operator is split into mean-field and small fluctuating components $\hat{\psi}(\mathbf{r},t) = \psi_{+\mathbf{k}_0}(\mathbf{r},t) + \psi_{-\mathbf{k}_0}(\mathbf{r},t) + \hat{\delta}(\mathbf{r},t)$. Here, $\psi_{\pm\mathbf{k}_0}(\mathbf{r},t)$ describes the two halves of the split condensate with centre-of-mass momenta $\pm\mathbf{k}_0$ respectively, whilst $\hat{\delta}(\mathbf{r},t)$ describes the scattered atoms. The Hamiltonian describing the fluctuating component $\hat{\delta}$, treated to the lowest order in perturbation theory, can be written in the form [1–3]

$$\hat{H} = \int d^3\mathbf{r}\left[-\frac{\hbar^2}{2m}\hat{\delta}^{\dagger}(\mathbf{r},t)\nabla^2\hat{\delta}(\mathbf{r},t) + 2U\psi^*_{+k_0}(\mathbf{r},t)\psi^*_{-k_0}(\mathbf{r},t)\hat{\delta}(\mathbf{r},t)^2 + h.c.\right], \tag{1}$$

where $U = 4\pi\hbar^2 a/m$ is the interaction strength characterised by the $s$-wave scattering length $a$. In the above Hamiltonian, we have additionally assumed that the mean-field interaction potential seen by the scattered atoms is much smaller than their mean kinetic energy so that the mean-field energy shifts can be safely ignored.

To invoke the undepleted pump approximation, corresponding to short collision durations such that the number of scattered atoms is only a small fraction of the source condensate, we consider an initial homogeneous BEC of fixed density $\rho_0$. With the mean kinetic energy of the colliding atoms being much larger than the mean-field interaction energy, the mean-field components $\psi_{\pm\mathbf{k}_0}(\mathbf{r},t)$ of the split condensate can be approximated by freely propagating fields [1, 2],

$$\psi_{\pm\mathbf{k}_0}(\mathbf{r},t) = \sqrt{\rho_0/2}\exp\left(\pm i\mathbf{k_0}\cdot\mathbf{r} - i\frac{\hbar|\mathbf{k}_0|^2}{2m}t\right). \tag{2}$$

Considering next the discrete (for a finite quantisation box) Fourier components $\hat{a}_{\mathbf{k}}$ of the fluctuating operator and solving the corresponding linear Heisenberg equations of motion resulting from the Hamiltonian (1), we find the solutions

$$\hat{a}_{\mathbf{k}}(t) = \alpha_{\mathbf{k}}(t)\hat{a}_{\mathbf{k}}(0) + \beta_{\mathbf{k}}(t)\hat{a}^{\dagger}_{-\mathbf{k}}(0), \tag{3}$$

$$\hat{a}^{\dagger}_{-\mathbf{k}}(t) = \beta^*_{\mathbf{k}}(t)\hat{a}_{\mathbf{k}}(0) + \alpha^*_{\mathbf{k}}(t)\hat{a}^{\dagger}_{-\mathbf{k}}(0), \tag{4}$$

where the coefficients are given by

$$\alpha_{\mathbf{k}}(t) = \left[\cosh\left(\sqrt{g^2-\Delta_k^2}\, t\right) - \frac{i\Delta_k}{\sqrt{g^2-\Delta_k^2}}\sinh\left(\sqrt{g^2-\Delta_k^2}\, t\right)\right]e^{i\frac{\hbar|\mathbf{k}_0|^2}{2m}t}, \tag{5}$$

$$\beta_{\mathbf{k}}(t) = \frac{-ig}{\sqrt{g^2-\Delta_k^2}}\ \sinh\left(\sqrt{g^2-\Delta_k^2}\, t\right)e^{i\frac{\hbar|\mathbf{k}_0|^2}{2m}t}, \tag{6}$$

with $g \equiv U\rho_0/\hbar$ and $\Delta_k \equiv \hbar|\mathbf{k}|^2/2m - \hbar|\mathbf{k}_0|^2/2m$. These solutions are physically valid in the short-time limit, corresponding in general to less than 10% depletion of the source condensate.

In this model, atom-atom correlations in the scattering halo can be completely characterised by

$$n_{\mathbf{k}}(t) = \langle\hat{a}^{\dagger}_{\mathbf{k}}(t)\hat{a}_{\mathbf{k}}(t)\rangle = |\beta_{\mathbf{k}}(t)|^2, \tag{7}$$

$$m_{\mathbf{k},-\mathbf{k}}(t) = \langle\hat{a}_{\mathbf{k}}(t)\hat{a}_{-\mathbf{k}}(t)\rangle = \alpha_{\mathbf{k}}(t)\beta_{\mathbf{k}}(t), \tag{8}$$

which are known as the normal and anomalous densities respectively.

Even though the undepleted pump approximation outlined here and the Bogoliubov approach used in the numerical simulations in the main text share the same property that they both assume a constant total number of atoms in the colliding source condensates, there is an important difference between the two approaches. While the simple analytic solutions obtained above assume that the condensate *densities* remain constant as well, the Bogoliubov approach does not impose this condition. Instead, it treats the expansion of the colliding condensates in free space as prescribed by the Gross-Pitaevskii equation for the mean-field component. This means that the Bogoliubov counterpart of the effective coupling $g = U\rho_0/\hbar$ introduced above (apart from being spatially dependent) becomes smaller with time as the condensate densities decrease during the expansion. Because of

this difference, the analytic results derived and discussed in these Supplementary Notes can only serve for qualitative insights into the physics behind the HOM effect for matter waves, but they will not necessarily be in quantitative agreement with the numerical results presented in the main text.

**Supplementary Note 2: Width of the HOM dip.** To estimate the width of the HOM dip after the application of Bragg pulses, we approximate the pulses as perfect mirrors and symmetric (50:50) beam-splitters over the relevant regions of the scattering halo, allowing us to model them as a series of simple linear transformations on the creation (annihilation) operators. Using Wick's theorem, we can then express the discrete-operator counterpart of the second-order correlation function considered in the main text, $g^{(2)}_{\rm RL}(t)=\langle:\hat{n}_{\rm R}(t)\hat{n}_{\rm L}(t):\rangle/\langle\hat{n}_{\rm R}(t)\rangle\langle\hat{n}_{\rm L}(t)\rangle$ at time $t_4$, purely in terms of the normal and anomalous densities at the end of the collision at time $t_1$,

$$g^{(2)}_{\rm RL}(t_4)=\frac{1}{2}+\frac{n_{\mathbf{k}_3}(t_1)^2+n_{\mathbf{k}_5}(t_1)^2}{\left(n_{\mathbf{k}_3}(t_1)+n_{\mathbf{k}_5}(t_1)\right)^2}+\frac{|m_{\mathbf{k}_3,\mathbf{k}_4}(t_1)|^2+|m_{\mathbf{k}_5,\mathbf{k}_6}(t_1)|^2}{2\left(n_{\mathbf{k}_3}(t_1)+n_{\mathbf{k}_5}(t_1)\right)^2}-\frac{m^*_{\mathbf{k}_3,\mathbf{k}_4}(t_1)m_{\mathbf{k}_5,\mathbf{k}_6}(t_1)e^{i\phi}+h.c.}{2\left(n_{\mathbf{k}_3}(t_1)+n_{\mathbf{k}_5}(t_1)\right)^2}, \tag{9}$$

where $\phi=\phi(\theta)\equiv 8\hbar|\mathbf{k}_0|^2\Delta t_{\rm free}\sin^2(\theta/2)/m$ and $\Delta t_{\rm free}$ is the duration of free-propagation after the $\pi$-pulse.

For the HOM dip minimum at $\theta=0$, this simple model predicts $g^{(2)}_{\rm RL}(t_4)=1$, whilst for sufficiently large $\theta$, such that the momenta $\mathbf{k}_{5,6}$ lie outside the scattering halo, we find $g^{(2)}_{\rm RL}(t_4)=2+1/2n_{\mathbf{k}_3}(t_1)$. For intermediate values of $\theta$, the full HOM dip profile is described by equation (9) and is shown in Supplementary Fig. 1 by the solid (red) curve. From the structure of equation (9), it is clear that the characteristic width of the dip will depend strongly on the widths of the densities $|m_{\mathbf{k}_5,\mathbf{k}_6}(t_1)|$ and $n_{\mathbf{k}_5}(t_1)$.

For a simple analytic estimate of the dip width we further approximate the radial profile of the halo density, equation (7), as well as of the anomalous moment, equation (8), which are both spherically symmetric, by Gaussian functions of the form $\propto\exp\left[-(k-k_0)^2/2\delta k_r^2\right]$, where $k\equiv|\mathbf{k}|$ and $\delta k_r$ is the rms width. The relevant densities are then given by

$$n_{\mathbf{k}_3}(t_1)=n_{\mathbf{k}_4}(t_1)=n_0, \tag{10}$$

$$n_{\mathbf{k}_5}(t_1)=n_{\mathbf{k}_6}(t_1)=n_0e^{-|\mathbf{k}_0|^2\left[1-\sqrt{5-4\cos(\theta)}\right]^2/2\delta k_r^2}, \tag{11}$$

$$|m_{\mathbf{k}_3,\mathbf{k}_4}(t_1)|=m_0, \tag{12}$$

$$|m_{\mathbf{k}_5,\mathbf{k}_6}(t_1)|=m_0e^{-|\mathbf{k}_0|^2\left[1-\sqrt{5-4\cos(\theta)}\right]^2/2\delta k_r^2}. \tag{13}$$

Here, $n_0$ is the peak occupancy predicted by equation (7) and $m_0=\sqrt{n_0(1+n_0)}$, where we have have used the identity $|m_{\mathbf{k},-\mathbf{k}}(t)|^2=n_{\mathbf{k}}(t)[1+n_{\mathbf{k}}(t)]$. To simplify our approximation of equation (9), we impose the condition Arg $[m^*_{\mathbf{k}_3,\mathbf{k}_4}(t_1)$ $m_{\mathbf{k}_5,\mathbf{k}_6}(t_1)e^{i\phi}]=0$, which amounts to ignoring any phase variations of the anomalous density across the scattering halo. Combined with equations (11) and (13), this simplification allows us to write equation (9) in the form

$$g^{(2)}_{\rm RL}(t_4)=\frac{1}{2}+\frac{1+n_0}{2n_0}\tanh^2\left(\beta(\theta)\right)+\frac{1}{{\rm sech}\left(\beta(\theta)\right)+1}, \tag{14}$$

where

$$\beta(\theta)\equiv\frac{|\mathbf{k}_0|^2\left[1-\sqrt{5-4\cos(\theta)}\right]^2}{2\delta k_r^2}. \tag{15}$$

The second-order correlation $g^{(2)}_{\rm RL}(t_4)$, equation (14), as a function of the angle $\theta$, has a full width at half maximum (FWHM) with respect to unity of

$$w_{dip}=2\ \arccos\left[\frac{5}{4}-\frac{1}{4}\left(1+\sqrt{\frac{2\delta k_r^2\beta_0}{|\mathbf{k}_0|^2}}\right)^2\right], \tag{16}$$

in units of radians, where

$$\beta_0\equiv\log\left(3+\frac{2\sqrt{1+2\left(1+\frac{1}{2n_0}\right)^2}}{1+\frac{1}{2n_0}}\right). \tag{17}$$

In Supplementary Fig. 1 we plot the envelope fit to the HOM dip profile, equation (14), as a dashed curve, which shows reasonable agreement with the full analytic result of equation (9) in terms of the overall shape of the dip. The discrepancies in the width of the dip are completely attributable to our assumption that $|m_{\mathbf{k}_5,\mathbf{k}_6}(t_1)|$ shares the same rms width as $n_{\mathbf{k}_5}(t_1)$, and our neglection of the phase profile Arg $[m^*_{\mathbf{k}_3,\mathbf{k}_4}(t_1)m_{\mathbf{k}_5,\mathbf{k}_6}(t_1)e^{i\phi}]$. The oscillations in the wings of equation (9) are due to a combination of this phase profile and oscillations in $n_{\mathbf{k}}(t_1)$ at the spontaneous noise level for $g^2-\Delta_k^2<0$ outside the scattering halo.

Lastly, by comparison of equation (9) to the phase-insensitive envelope fit in Supplementary Fig. 1, it is clear that the oscillations in the wings of equation (9) are centred on a mean-value $\overline{g^{(2)}_{\mathrm{RL}}(t_4)}=2+1/2n_{\mathbf{k}_3}(t_1)$. This observation justifies our definition of dip visibility employed in the main text.

**Supplementary Note 3: Relation between HOM effect and Cauchy-Schwarz inequality.** The quantum nature of the Hong-Ou-Mandel effect is commonly characterised by the visibility of the HOM dip. In this section we outline the relation between this visibility and the violation of the Cauchy-Schwarz (CS) inequality, which has been demonstrated in condensate collisions in Refs. [4, 5].

The visibility of the HOM dip is defined as $V=1-\min[g^{(2)}_{\mathrm{RL}}(t_4)]/\max[g^{(2)}_{\mathrm{RL}}(t_4)]$, where $\min[g^{(2)}_{\mathrm{RL}}(t_4)]$ occurs for $\theta=0$ and $\max[g^{(2)}_{\mathrm{RL}}(t_4)]$ corresponds to sufficiently large $\theta$ such that momenta $\mathbf{k}_{5,6}$ lie outside the scattering halo. To highlight the link to the CS inequality we evaluate these quantities by rewriting (9) in terms of the second-order correlations $g^{(2)}_{\mathbf{k},\mathbf{k}'}(t)=\langle\hat{a}^\dagger_{\mathbf{k}}(t)\hat{a}^\dagger_{\mathbf{k}'}(t)\hat{a}_{\mathbf{k}'}(t)\hat{a}_{\mathbf{k}}(t)\rangle/\langle\hat{a}^\dagger_{\mathbf{k}}(t)\hat{a}_{\mathbf{k}}(t)\rangle\langle\hat{a}^\dagger_{\mathbf{k}'}(t)\hat{a}_{\mathbf{k}'}(t)\rangle$ at the end of the collision at time $t_1$,

$$\min[g^{(2)}_{\mathrm{RL}}(t_4)]=\frac{1}{2}g^{(2)}_{\mathbf{k}_3\mathbf{k}_3}(t_1),\tag{18}$$

$$\max[g^{(2)}_{\mathrm{RL}}(t_4)]=\frac{1}{2}\left[g^{(2)}_{\mathbf{k}_3\mathbf{k}_4}(t_1)+g^{(2)}_{\mathbf{k}_3\mathbf{k}_3}(t_1)\right],\tag{19}$$

where we use the symmetry $g^{(2)}_{\mathbf{k}_3\mathbf{k}_3}(t_1)=g^{(2)}_{\mathbf{k}_4\mathbf{k}_4}(t_1)$.

The CS inequality, in the context of the correlations after the collision, is given as $g^{(2)}_{\mathbf{k}_i,\mathbf{k}_j}(t_1)\leq\sqrt{g^{(2)}_{\mathbf{k}_i,\mathbf{k}_i}(t_1)g^{(2)}_{\mathbf{k}_j,\mathbf{k}_j}(t_1)}$, where we assume $n_{\mathbf{k}_i}(t_1)=n_{\mathbf{k}_j}(t_1)$. We characterise a violation of the inequality by the quantity $C=g^{(2)}_{\mathbf{k}_i,\mathbf{k}_j}(t_1)/\sqrt{g^{(2)}_{\mathbf{k}_i,\mathbf{k}_i}(t_1)g^{(2)}_{\mathbf{k}_j,\mathbf{k}_j}(t_1)}$ $>1$. Using this and equations (18) and (19) we may quantify the visibility of the HOM dip as

$$V=1-\frac{1}{1+C}.\tag{20}$$

A measurement of $V>0.5$ corresponds strictly to $C>1$ and thus a violation of the inequality, implying the correlations between scattered atom pairs cannot be described by classical stochastic random variables [6].

**Supplementary Note 4: Effects of realistic Bragg pulses.** In the qualitative description of our model and the simplified undepleted pump description, we assume perfect $\pi$ and $\pi$/2-pulses for all momentum components which are coupled (i.e., 100% and 50% transfer of atomic populations respectively). However, such perfect transfer only occurs for the momentum components, $\mathbf{k}_1$ and $\mathbf{k}_2$ (corresponding to $\theta=0$), specifically targeted by the Bragg pulse, which satisfy the Bragg resonance condition for momentum and energy conservation. For $|\theta|>0$, on the other hand, the coupled components $\mathbf{k}_{3(4)}$ and $\mathbf{k}_{6(5)}$ do not conserve energy and are detuned from this resonance condition, leading to a population transfer varying from the canonical definition of $\pi$ and $\pi$/2-pulses. In this section we investigate the quantitative effects such off-resonant coupling has on the nature of the HOM dip.

For a simple insight we model the case of square Bragg pulses where the lattice depth is ramped on/off instantaneously, $V_L(t)=V_0\Theta(t-t_{\mathrm{on}})[1-\Theta(t-t_{\mathrm{off}})]$ where $\Theta$ is the Heaviside step function, and restrain coupling to momentum components separated by a single momentum kick, $\mathbf{k}_{i,j}$ where $\mathbf{k}_j=\mathbf{k}_i-2\mathbf{k}_L$. A $\pi$-pulse is defined by the duration $\tau_\pi=2\pi\hbar/V_0$ and a $\pi$/2-pulse by $\tau_{\pi/2}=\pi\hbar/V_0$. This model can be solved analytically (see, e.g. Ref. [7]) to give the transmission and reflection amplitudes of the pulses, and is a reasonably valid approximation to the Gaussian Bragg pulses used in numerical simulations. To compare directly we note that square and Gaussian Bragg pulses of the same lattice depth and of duration $\tau$ and $\tau'$ respectively are related by the equivalence relation $\tau=\sqrt{2\pi}\tau'$.

The collision process is again treated according to the undepleted pump model outlined in Supplementary Note 1; in Supplementary Fig. 1 we plot the resulting $g^{(2)}_{\mathrm{RL}}(t_4)$ for the case of realistic Bragg pulses as a dash-dotted (green) curve. We choose $\tau_\pi=\tau_{\pi/2}=\sqrt{2\pi}\tau'$ where $\tau'=2.5$ $\mu$s matches the pulse duration used in the simulations of the main text. For small $\theta$ we find little deviation from calculations based on perfect mirror/beam-splitter transformations [shown as the solid (red) curve]; the overall shape of the dip is preserved, although there is a slight decrease in the FWHM. For large $\theta$ the effects of the off-resonant coupling become larger, resulting in a decrease in period and amplitude of the oscillations in the wings of $g^{(2)}_{\mathrm{RL}}(t_4)$. In addition,

we observe the mean value in the wings, $\overline{g^{(2)}_{\rm RL}(t_4)}$, increases slightly, relative to the case of perfect mirror/beam-splitter transformations. However, the increase is sufficiently small so as not to affect our claim of a nonclassical visibility $V > 0.5$.

**Supplementary Note 5: Impact of realistic Bragg pulses on path distinguishability.** Beyond the quantitative changes to the structure of the HOM dip, another issue arising from off-resonant coupling relates to the treatment of path distinguishability in the scheme. In the archetypal optical HOM effect, perfect suppression of correlations between opposing output ports of the interferometer occurs only for symmetric (50:50) beam-splitters. In practice, asymmetry in the beam-splitter reflection/transmission ($R$/$T$) amplitudes provides which-way information (path distinguishability), leading to a decrease in dip visibility [8]. In this section we investigate how off-resonant coupling plays a similar role in our proposed scheme and seek to quantify the impact it may have on the visibility of the HOM dip.

In the qualitative analysis of our model, we observe that the inhomogeneous density of the scattering halo is pivotal to revealing the structure of the HOM dip. When atomic populations in components $\mathbf{k}_3$ and $\mathbf{k}_4$ are coupled to vacuum outside the populated region of the scattering halo (components $\mathbf{k}_6$ and $\mathbf{k}_5$ respectively), the paths through the beam-splitter are completely distinguishable. Such coupling corresponds to large $\theta$, where we have demonstrated the detuning from Bragg resonance has appreciable effects. In principle, if the detuning from perfect Bragg resonance is sufficiently large such that our $\pi$/2-pulse corresponds to $|R|^2 = 1$ and $|T|^2 = 0$ (or vice versa) for the off-resonant components, the visibility of the HOM dip would be completely attributable to which-way information gained from the off-resonant coupling rather than the inhomogeneous profile of the scattering halo.

To quantify the distinguishability provided by off-resonant coupling separately to that produced by the non-uniform scattering halo, we consider an artificial model describing the scattered atoms, wherein we remove all spatial structure from equations (7) and (8). The normal and anomalous densities are then completely characterised by

$$n_{\mathbf{k}}(t) = n_0, \tag{21}$$

$$m_{\mathbf{k},-\mathbf{k}}(t) = -i\sqrt{n_0(1+n_0)}, \tag{22}$$

where $n_0$ is the average occupation of the modes, chosen to match the peak of equation (7). We preserve the relation $|m_{\mathbf{k},-\mathbf{k}}(t)|^2 = n_{\mathbf{k}}(t)[1 + n_{\mathbf{k}}(t)]$ and for definiteness we have chosen the phase of the anomalous density to match that of equation (8) for $\Delta_k = 0$. To be consistent with this choice of phase profile, we also neglect any free-propagation effects in this calculation.

In Supplementary Fig. 2 we plot the maximum visibility of the HOM dip for the case of a uniform halo and taking into account the off-resonant coupling of both the $\pi$ and $\pi$/2-pulses (following the analytic treatment of Supplementary Note 4, compared to that expected for an inhomogeneous halo with perfect mirror/beam-splitter transformations (dashed line). As the visibility measure is sensitive to the mode occupation, we choose $n_0 \simeq 0.14$ to match the numerical results of the main text. We find that shorter pulse durations limit the effects of off-resonant coupling, which is in agreement with the results of Ref. [7] where the efficiency of transfer over a broad momentum width is found to decrease with pulse duration. It is also clear in Supplementary Fig. 2 that the maximum visibility due to off-resonant coupling cannot match that expected from an inhomogeneous halo for any $\tau$ investigated. The remaining small difference between the two curves at large $\tau$ is due to our modelling of imperfect mirrors, in addition to imperfect beam-splitter.

For the Gaussian pulse scheme used in the main text ($\tau' = 2.5$ $\mu$s) we calculate worst-case reflection amplitudes of $|R_\pi|^2 \simeq 0.84$ and $|R_{\pi/2}|^2 \simeq 0.43$ for the $\pi$ and $\pi$/2-pulses respectively, corresponding to $|\theta| = \pi/4$. The which-way information gained from this is predicted to give a visibility of 70%, compared to 82% for an inhomogeneous halo. This may seem large, however, it is important to note that this only corresponds to a maximal correlation of $g^{(2)}_{\rm RL}(t_4) \simeq 0.62\ (2 + 1/2n_0)$ (see Supplementary Fig. 2), whereas for an inhomogeneous scattering halo we expect an average value of $g^{(2)}_{\rm RL}(t_4) = 2 + 1/2n_0$ for large $|\theta|$. We thus conclude that, for the parameter regime simulated, full distinguishability of the paths through the interferometer and hence the magnitude of the dip visibility cannot be purely explained as a consequence of off-resonant coupling, but requires the inhomogeneity of the scattering halo to be taken into account.

## Supplementary References


[1] Ziń, P., Chwedeńczuk, J. & Trippenbach, M. Elastic scattering losses from colliding Bose-Einstein condensates. *Phys. Rev. A* **73**, 033602 (2006).

[2] Ogren, M. & Kheruntsyan, K. V. Atom-atom correlations in colliding Bose-Einstein condensates. *Phys. Rev. A.* **79**, 021606 (2009).

[3] Deuar, P., Chwedeńczuk, J., Trippenbach, M. & Ziń, P. Bogoliubov dynamics of condensate collisions using the positive-$P$ representation. *Phys. Rev. A* **83**, 063625 (2011).

[4] Kheruntsyan, K. V. *et al.* Violation of the Cauchy-Schwarz inequality with matter waves. *Phys. Rev. Lett.* **108**, 260401 (2012).
[5] Jaskula, J. *et al.* Sub-Poissonian number differences in four-wave mixing of matter waves. *Phys. Rev. Lett.* **105**, 190402 (2010).
[6] Su, C. & Wódkiewicz, K. Quantum versus stochastic or hidden-variable fluctuations in two-photon interference effects. *Phys. Rev. A* **44**, 6097–6108 (1991).
[7] Szigeti, S. S., Debs, J. E., Hope, J. J., Robins, N. P. & Close, J. D. Why momentum width matters for atom interferometry with bragg pulses. *New Journal of Physics* **14**, 023009 (2012).
[8] Hong, C. K., Ou, Z. Y. & Mandel, L. Measurement of subpicosecond time intervals between two photons by interference. *Phys. Rev. Lett.* **59**, 2044–2046 (1987).
